# Supplementary material for: Collaborative Vision-Text Representation Optimizing for Open-Vocabulary Segmentation
Source: arXiv:2408.00744 source file (2024-12-04)
Supplement: Supplementary file 1 [file appendix-vis-1.pdf]

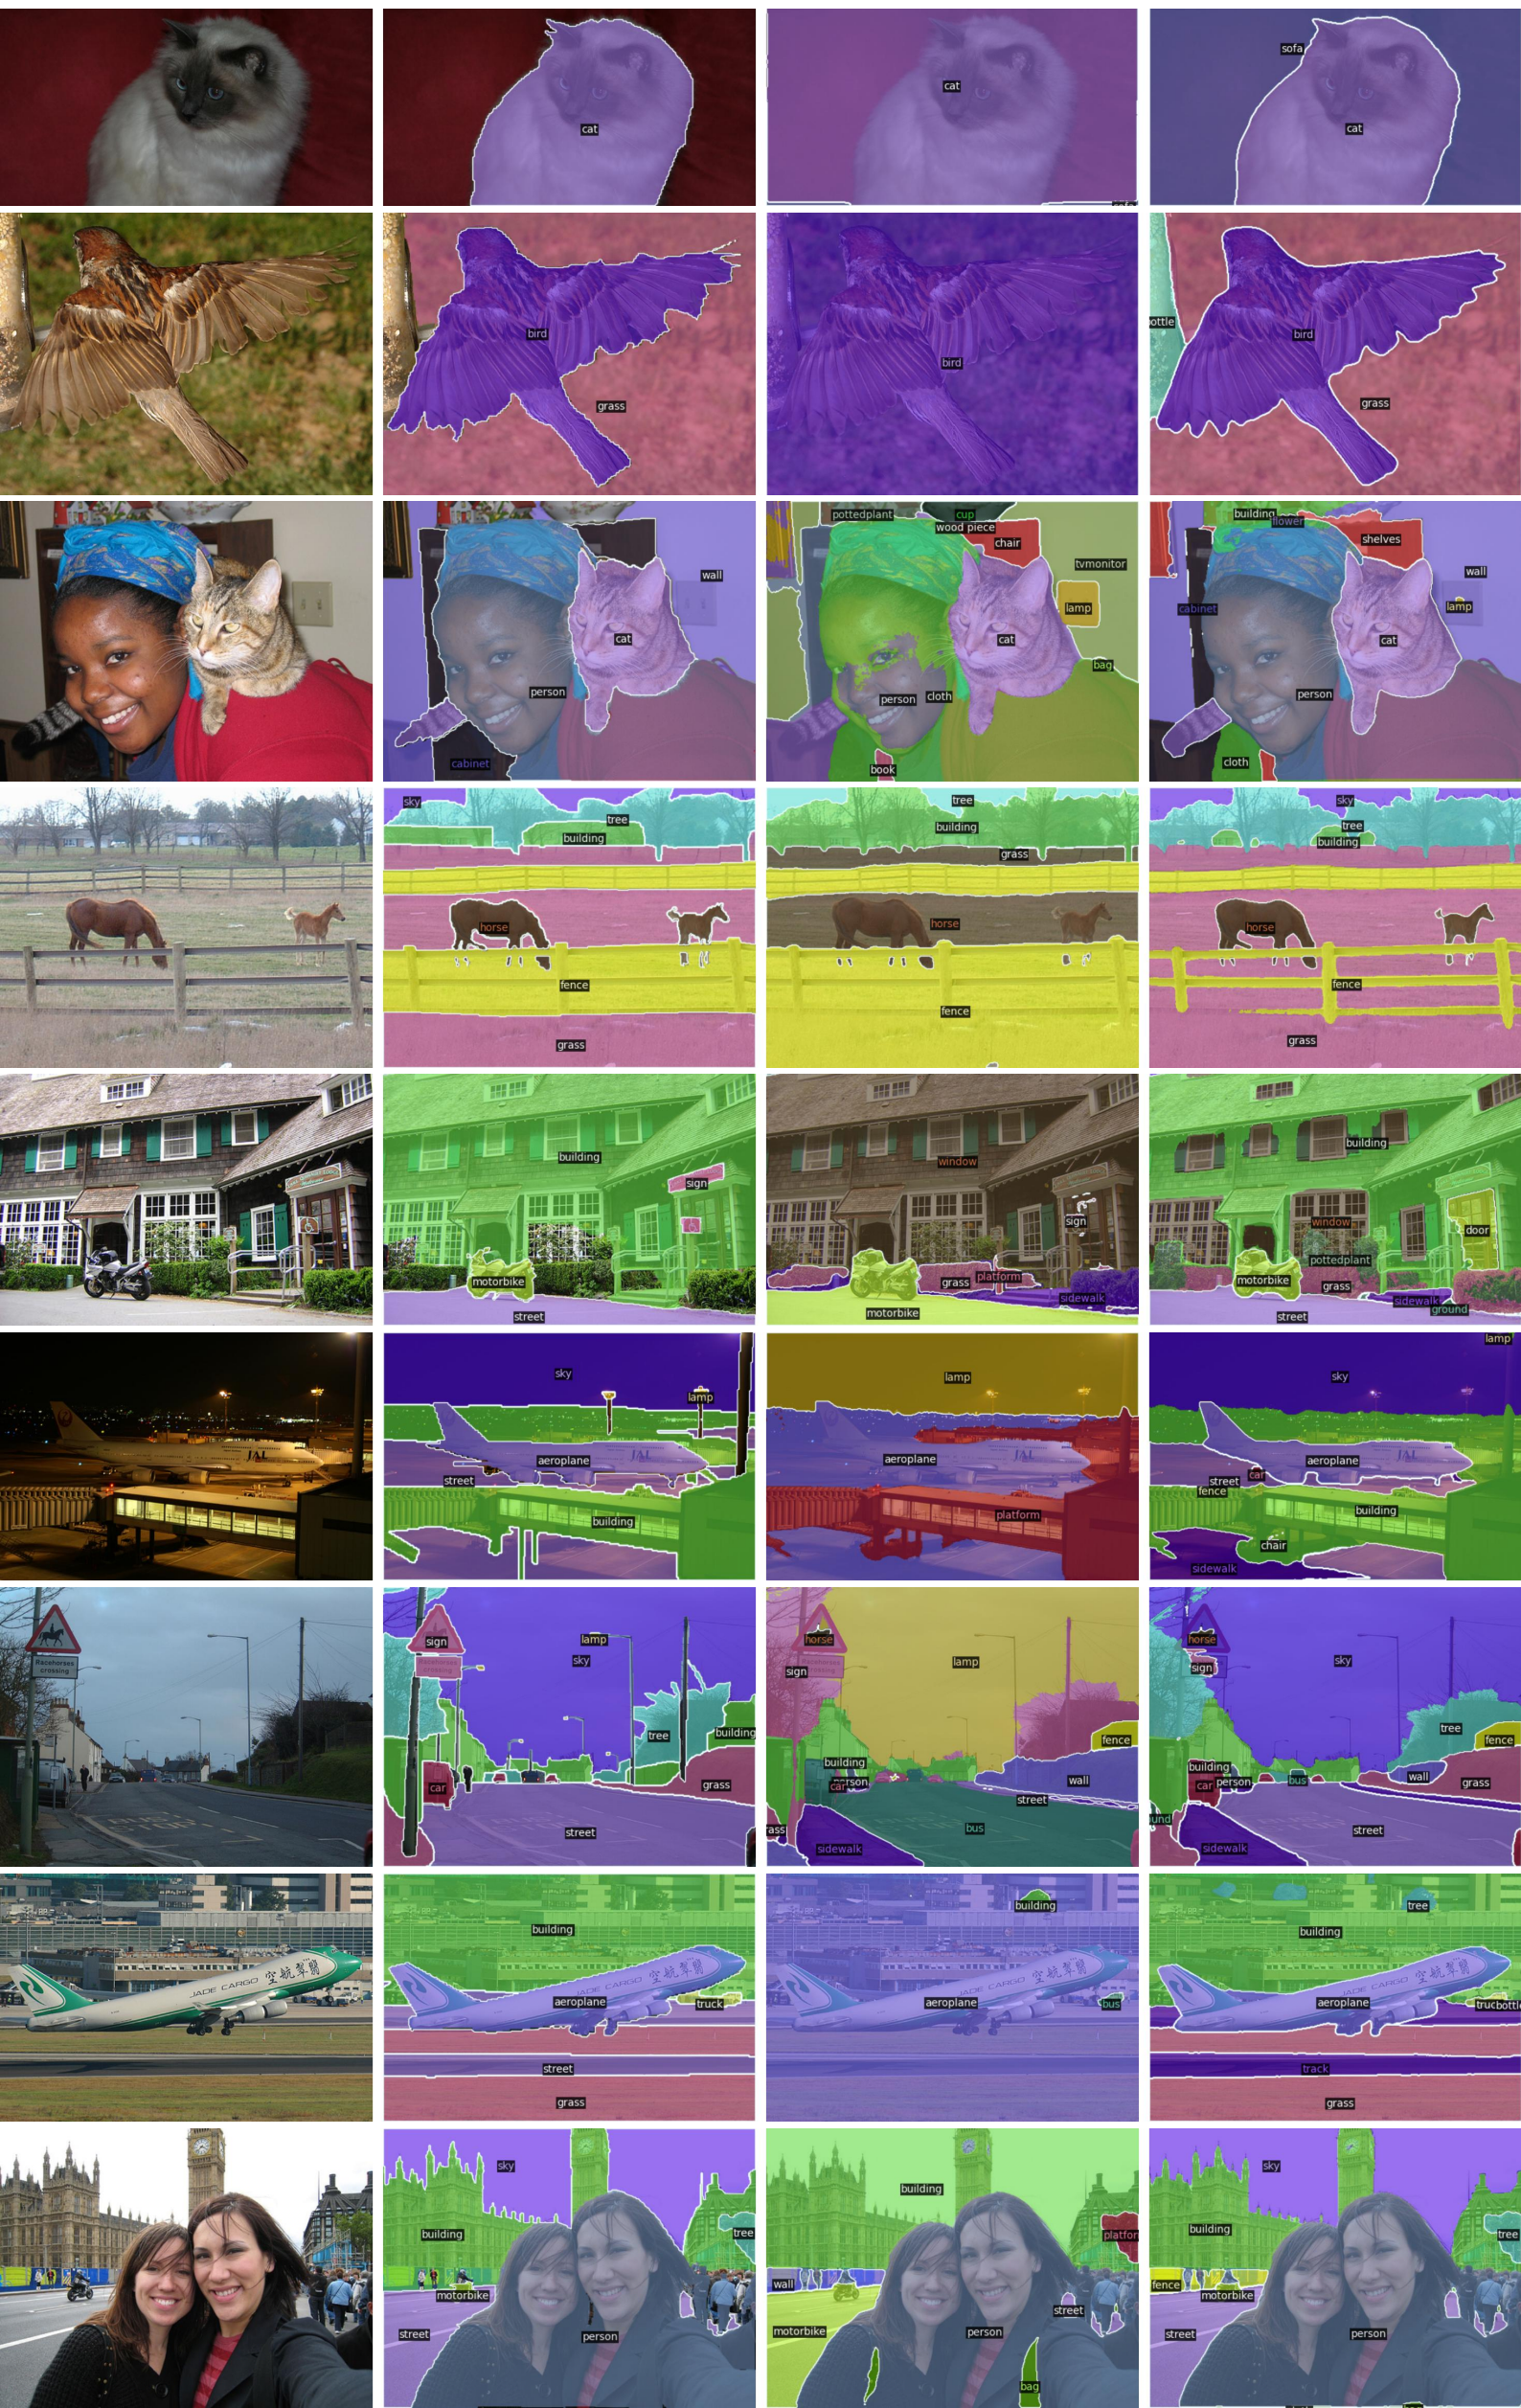

Image

GT

frozen CLIP

Fine-tuned CLIP
